# Supplementary material for: Data-driven Simulation and Optimization for Covid-19 Exit Strategies
Source: arXiv:2006.07087 source file (2020-06-12)
Supplement: Supplementary file 1 [file appendix.tex]

\clearpage
\section{Appendix}
\label{section:appendix}

\begin{table}[h]
\centering
\begin{tabular}{r||r|r|r|}
Country & SEIR deaths ($R_t$ as of 15-02-2020) & DN-SEIR deaths (with NPIs) & True deaths\\
\hline
Belgium & 2,180 & 7,049 [6,996-7,112] & 7,501 \\
France &  30,382 & 25,493 [25,314-25,695] & 24,087\\
Germany & 48,724 & 7,293 [7,242-7,353] &6,115 \\
Greece &  107 & 107 [106-108] & 139 \\
Italy & 230,989 & 22,476 [22,348-22,623] & 27,682\\
Latvia & 32 & 32 [32-33] & 15\\
Luxembourg & 78 & 78 [78-79] & 89\\
Netherlands & 3,364 & 3,348 [3,317-3,384] &4,711 \\
Spain  & 81,347 & 19,449 [19,338-19,577] & 24,543\\
Switzerland & 1,391 & 1,390 [1,383-1,399] & 1,716 \\

\hline
\hline
Brazil &  2.358 & 2,359 [2,312-2,414] &5,466\\
Cameroon &  30 & 30 [29-31] & 61\\
Canada & 1,106 & 2,047 [2,011-2,088] & 2,996\\
Japan & 363 & 505 [498-512] & 415\\
United Kingdom & 22,703 & 19,882 [19,659-20,086] & 26,771\\
\end{tabular}
\caption{Total deaths on April 29th as predicted by the DN-SEIR model and the actual deahs. We compare the numbers with the predicted one by a SEIR model using the Reproduction rate of each country on February 15th.}
\label{table:shortterm_fitting_death}
\end{table}

\begin{figure}[h]
\centering
\includegraphics[width=0.8\linewidth]{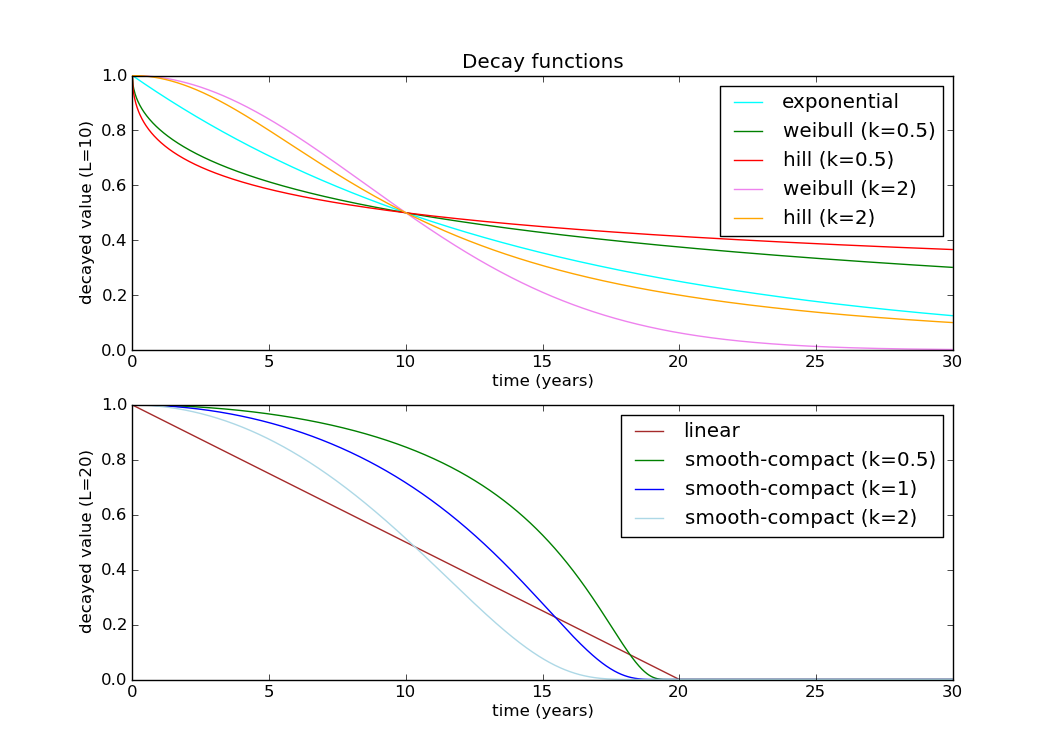}
\caption{Various decay functions with L=10 and L=20 }
\label{fig:decay_functions}
\vspace{-1.0em}
\end{figure}

\begin{figure}[h]
\centering
\includegraphics[width=\linewidth]{figures/fit/c1.png}
\caption{Predicted cases, hospitalizations, critical and deaths of our fitted model for Belgium.}
\label{fig:viz_c1_shortterm}
\vspace{-1.0em}
\end{figure}

\begin{figure}[h]
\centering
\includegraphics[width=\linewidth]{figures/fit/c2.png}
\caption{Predicted cases, hospitalizations, critical and deaths of our fitted model for France.}
\label{fig:viz_c2_shortterm}
\vspace{-1.0em}
\end{figure}

\begin{figure}[h]
\centering
\includegraphics[width=\linewidth]{figures/fit/c3.png}
\caption{Predicted cases, hospitalizations, critical and deaths of our fitted model for Germany.}
\label{fig:viz_c3_shortterm}
\vspace{-1.0em}
\end{figure}

\begin{figure}[h]
\centering
\includegraphics[width=\linewidth]{figures/fit/c4.png}
\caption{Predicted cases, hospitalizations, critical and deaths of our fitted model for Greece.}
\label{fig:viz_c4_shortterm}
\vspace{-1.0em}
\end{figure}

\begin{figure}[h]
\centering
\includegraphics[width=\linewidth]{figures/fit/c5.png}
\caption{Predicted cases, hospitalizations, critical and deaths of our fitted model for Italy.}
\label{fig:viz_c5_shortterm}
\vspace{-1.0em}
\end{figure}

\begin{figure}[h]
\centering
\includegraphics[width=\linewidth]{figures/fit/c6.png}
\caption{Predicted cases, hospitalizations, critical and deaths of our fitted model for Latvia.}
\label{fig:viz_c6_shortterm}
\vspace{-1.0em}
\end{figure}

\begin{figure}[h]
\centering
\includegraphics[width=\linewidth]{figures/fit/c8.png}
\caption{Predicted cases, hospitalizations, critical and deaths of our fitted model for Netherlands.}
\label{fig:viz_c8_shortterm}
\vspace{-1.0em}
\end{figure}

\begin{figure}[h]
\centering
\includegraphics[width=\linewidth]{figures/fit/c9.png}
\caption{Predicted cases, hospitalizations, critical and deaths of our fitted model for Spain.}
\label{fig:viz_c9_shortterm}
\vspace{-1.0em}
\end{figure}

\begin{figure}[h]
\centering
\includegraphics[width=\linewidth]{figures/fit/c10.png}
\caption{Predicted cases, hospitalizations, critical and deaths of our fitted model for Switzerland.}
\label{fig:viz_c10_shortterm}
\vspace{-1.0em}
\end{figure}

\begin{figure}[h]
\centering
\includegraphics[width=\linewidth]{figures/fit/c11.png}
\caption{Predicted cases, hospitalizations, critical and deaths of our fitted model for Brazil.}
\label{fig:viz_c1_shortterm}
\vspace{-1.0em}
\end{figure}

\begin{figure}[h]
\centering
\includegraphics[width=\linewidth]{figures/fit/c12.png}
\caption{Predicted cases, hospitalizations, critical and deaths of our fitted model for Cameroon.}
\label{fig:viz_c12_shortterm}
\vspace{-1.0em}
\end{figure}

\begin{figure}[h]
\centering
\includegraphics[width=\linewidth]{figures/fit/c13.png}
\caption{Predicted cases, hospitalizations, critical and deaths of our fitted model for Canada.}
\label{fig:viz_c13_shortterm}
\vspace{-1.0em}
\end{figure}

\begin{figure}[h]
\centering
\includegraphics[width=\linewidth]{figures/fit/c14.png}
\caption{Predicted cases, hospitalizations, critical and deaths of our fitted model for Japan.}
\label{fig:viz_c14_shortterm}
\vspace{-1.0em}
\end{figure}

\begin{figure}[h]
\centering
\includegraphics[width=\linewidth]{figures/fit/c15.png}
\caption{Predicted cases, hospitalizations, critical and deaths of our fitted model for United Kingdom.}
\label{fig:viz_c15_shortterm}
\vspace{-1.0em}
\end{figure}
